# Supplementary material for: Cross-TOP: Zero-Shot Cross-Schema Task-Oriented Parsing
Source: arXiv:2206.05352 source file (2022-06-10)
Supplement: Supplementary file 1 [file appendix.tex]

\section*{Appendix}

\section{Mechanical Turk Instructions}\label{appendix:mturk}
The instructions given to the worker were tempalted as shown in Figure \ref{fig:MturkInstructions}.  

The tasks can be descibed as a natural language text generation with constrained menu. The number of responses was limited to 3 submission per worker to balance diversity of responses and reponsiveness ratios.

\medskip

Overall we collected answers form about 60 distinc workers for \textsc{burger},  \textsc{sub} and  \textsc{coffee} and about 90 for \textsc{burrito}. All dataset together we have data from 183 unique individuals.

\medskip

\begin{figure*}[b]
	
	\begin{note}
	\scriptsize
	Suppose you want to place your usual order at your favorite \emph{type of restaurant}  (like \emph{examples of such venues}) for you, your partner, your family or your group of friends. 
	Your task is to enter your order exactly as you would say it, verbatim, when you place the order at that restaurant.

	\medskip

	IMPORTANT: This restaurant has a limited menu provided below. Only order items available on the menu, but do so with the same words you usually use when ordering these items:
	
	\medskip
	
	\begin{center}
	 \emph{*** Picture of restaurant Menu ***}
	\end{center}

		\medskip
	
	Write as you would speak. Make sure that:
	\begin{itemize}
	 \item you write your order exactly as you would say it
	 \item your usual order may include many items and if so, include them all when you enter your order below
   	\item if you complete multiple HITs, vary the type of orders you place. The orders should be usual orders you, your friends or family place, but with varying number or types of items, toppings, sides or drinks.
	\end{itemize}

	\medskip
	Enter your order below, using the limited menu above, exactly as you would say it at the restaurant :

	\medskip	
	
	\begin{center}
	 \emph{*** Type order here ***}
	\end{center}

	\medskip

	How many times per month do you order at/from a Burrito Restaurant? \emph{*** cursor selection ***}
	
	\end{note}
\caption{Template prompt given to Mechanical Turk workers, common across all 4 tasks. The only significant attribute varying accross tasks was the vailable menu to order from.}\label{fig:MturkInstructions}

\end{figure*}

The menu provided for each collection are given in Figure \ref{fig:allMenus}:  \textsc{burrito} (top-left), \textsc{Sub} (top-right), \textsc{Burger} (bottom-left) and \textsc{coffee} (bottom-right).

\begin{figure*}[b]
	\centering
	\begin{subfigure}[b]{0.475\textwidth}
	\includegraphics[width=\textwidth]{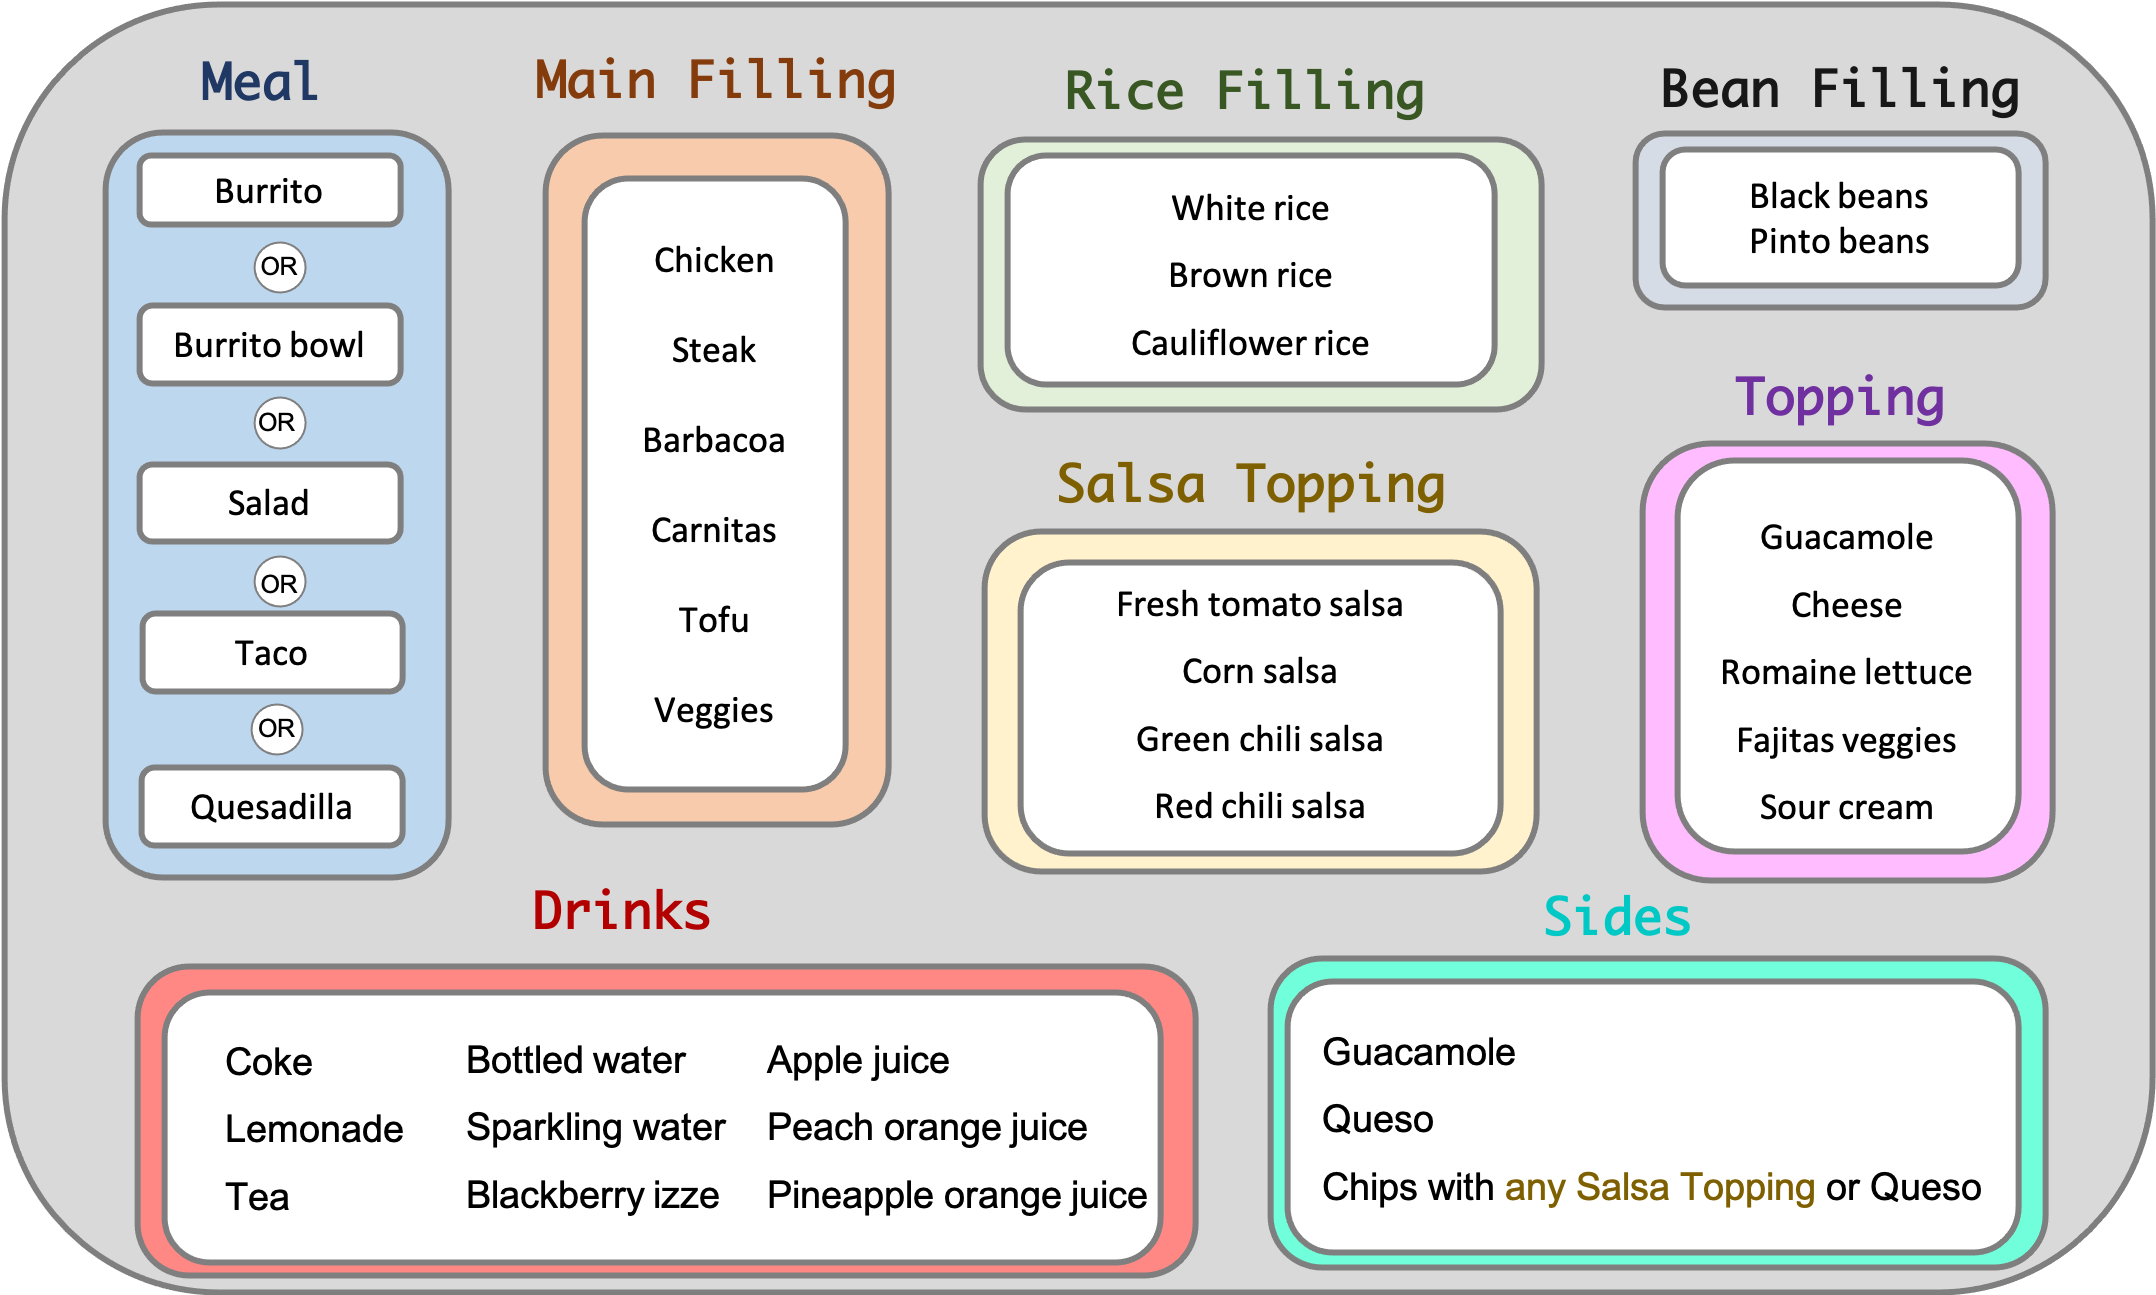}
	\end{subfigure}
	\hfill
	\begin{subfigure}[b]{0.475\textwidth}
	\includegraphics[width=\textwidth]{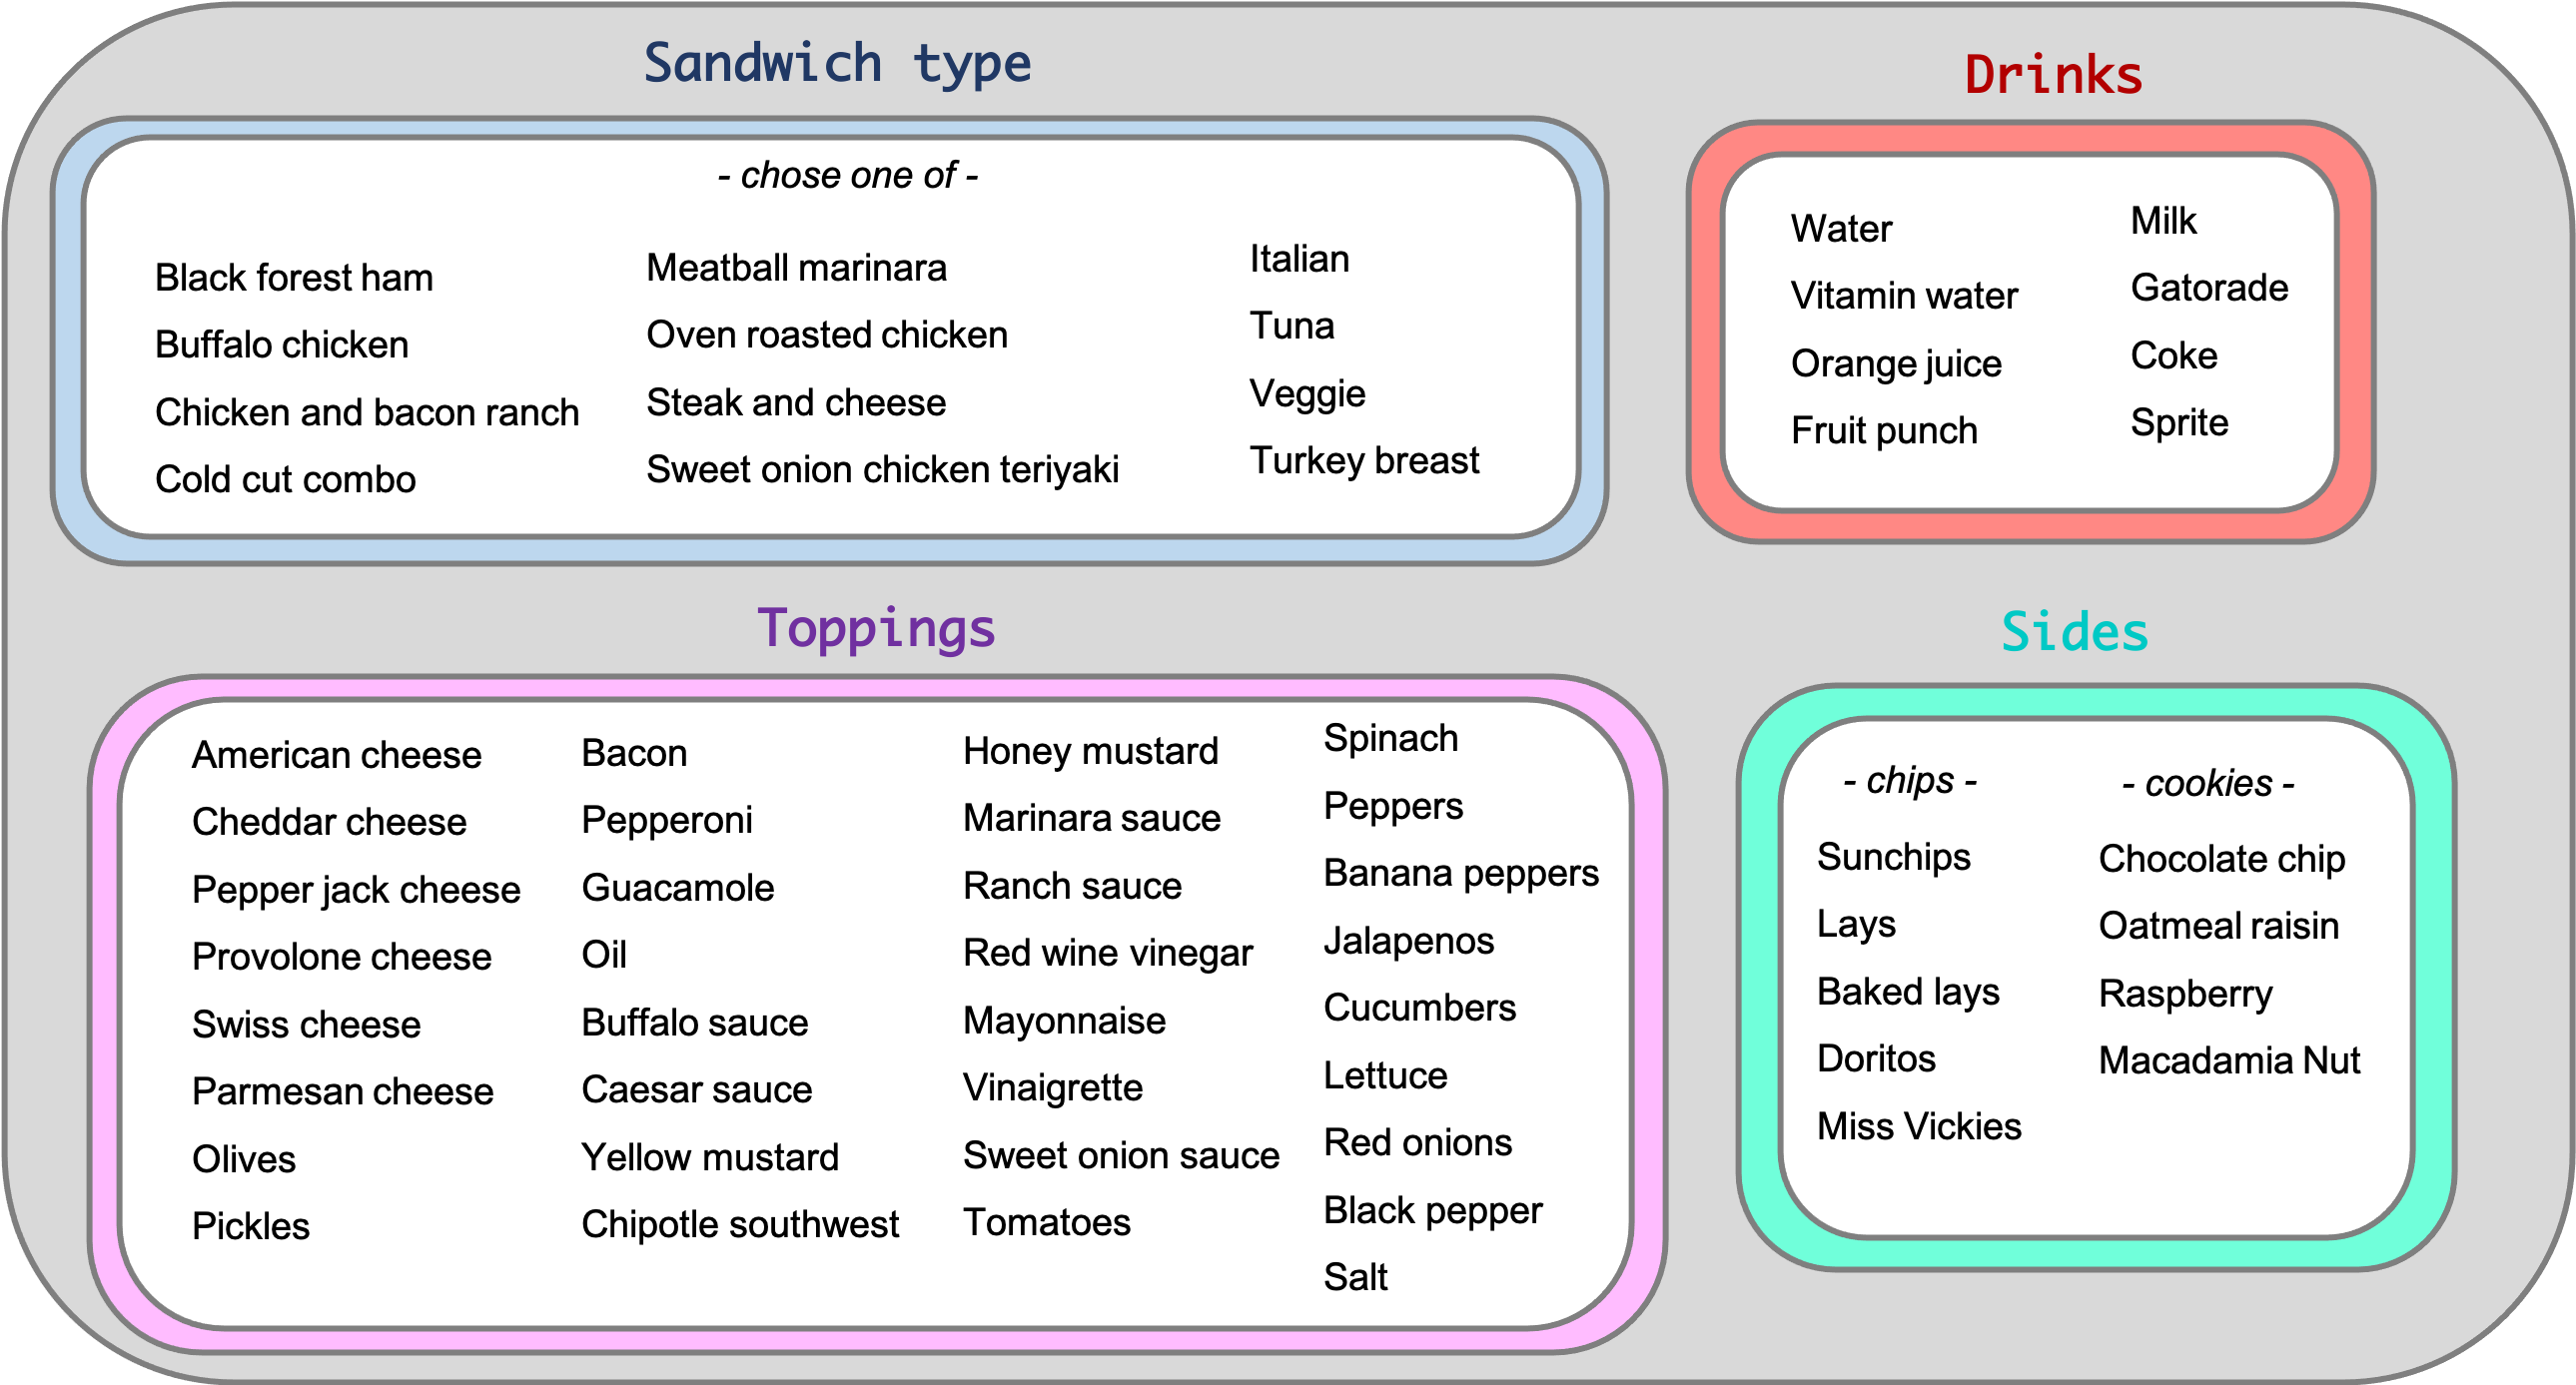}
	\end{subfigure}
	\vskip\baselineskip
	\begin{subfigure}[b]{0.475\textwidth}
	\includegraphics[width=\textwidth]{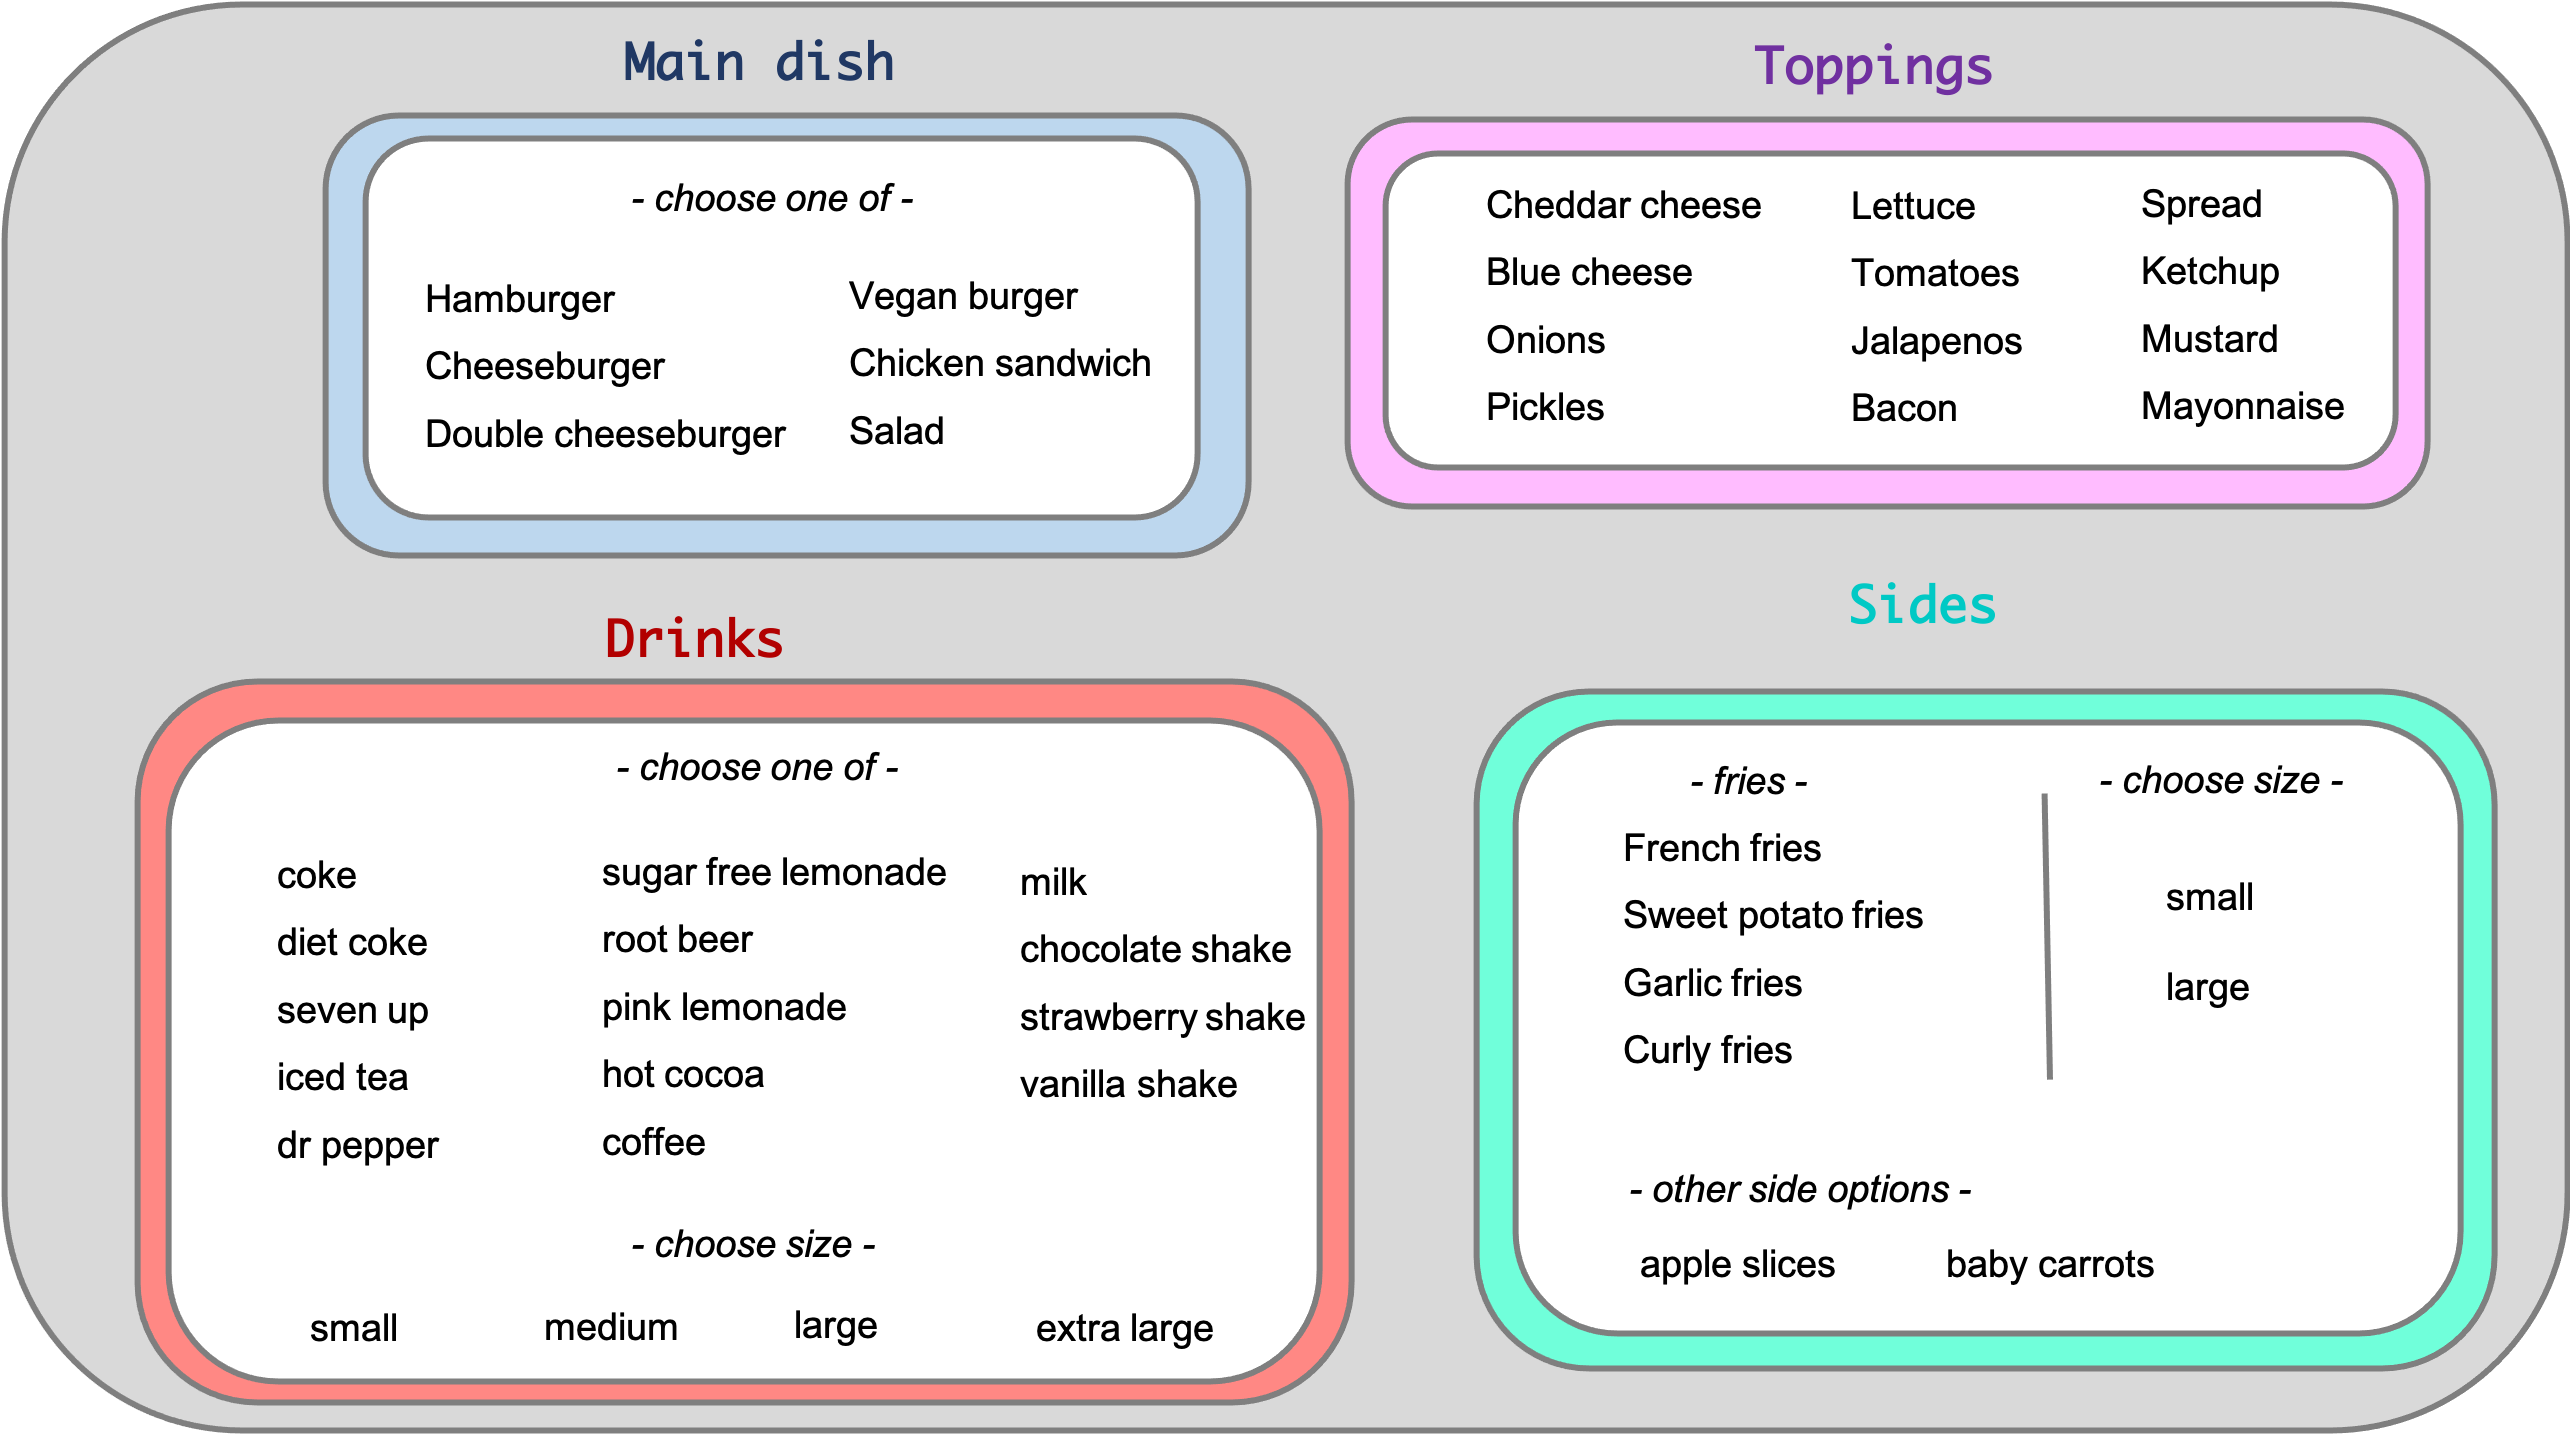}
	\end{subfigure}
	\hfill
	\begin{subfigure}[b]{0.475\textwidth}
	\includegraphics[width=\textwidth]{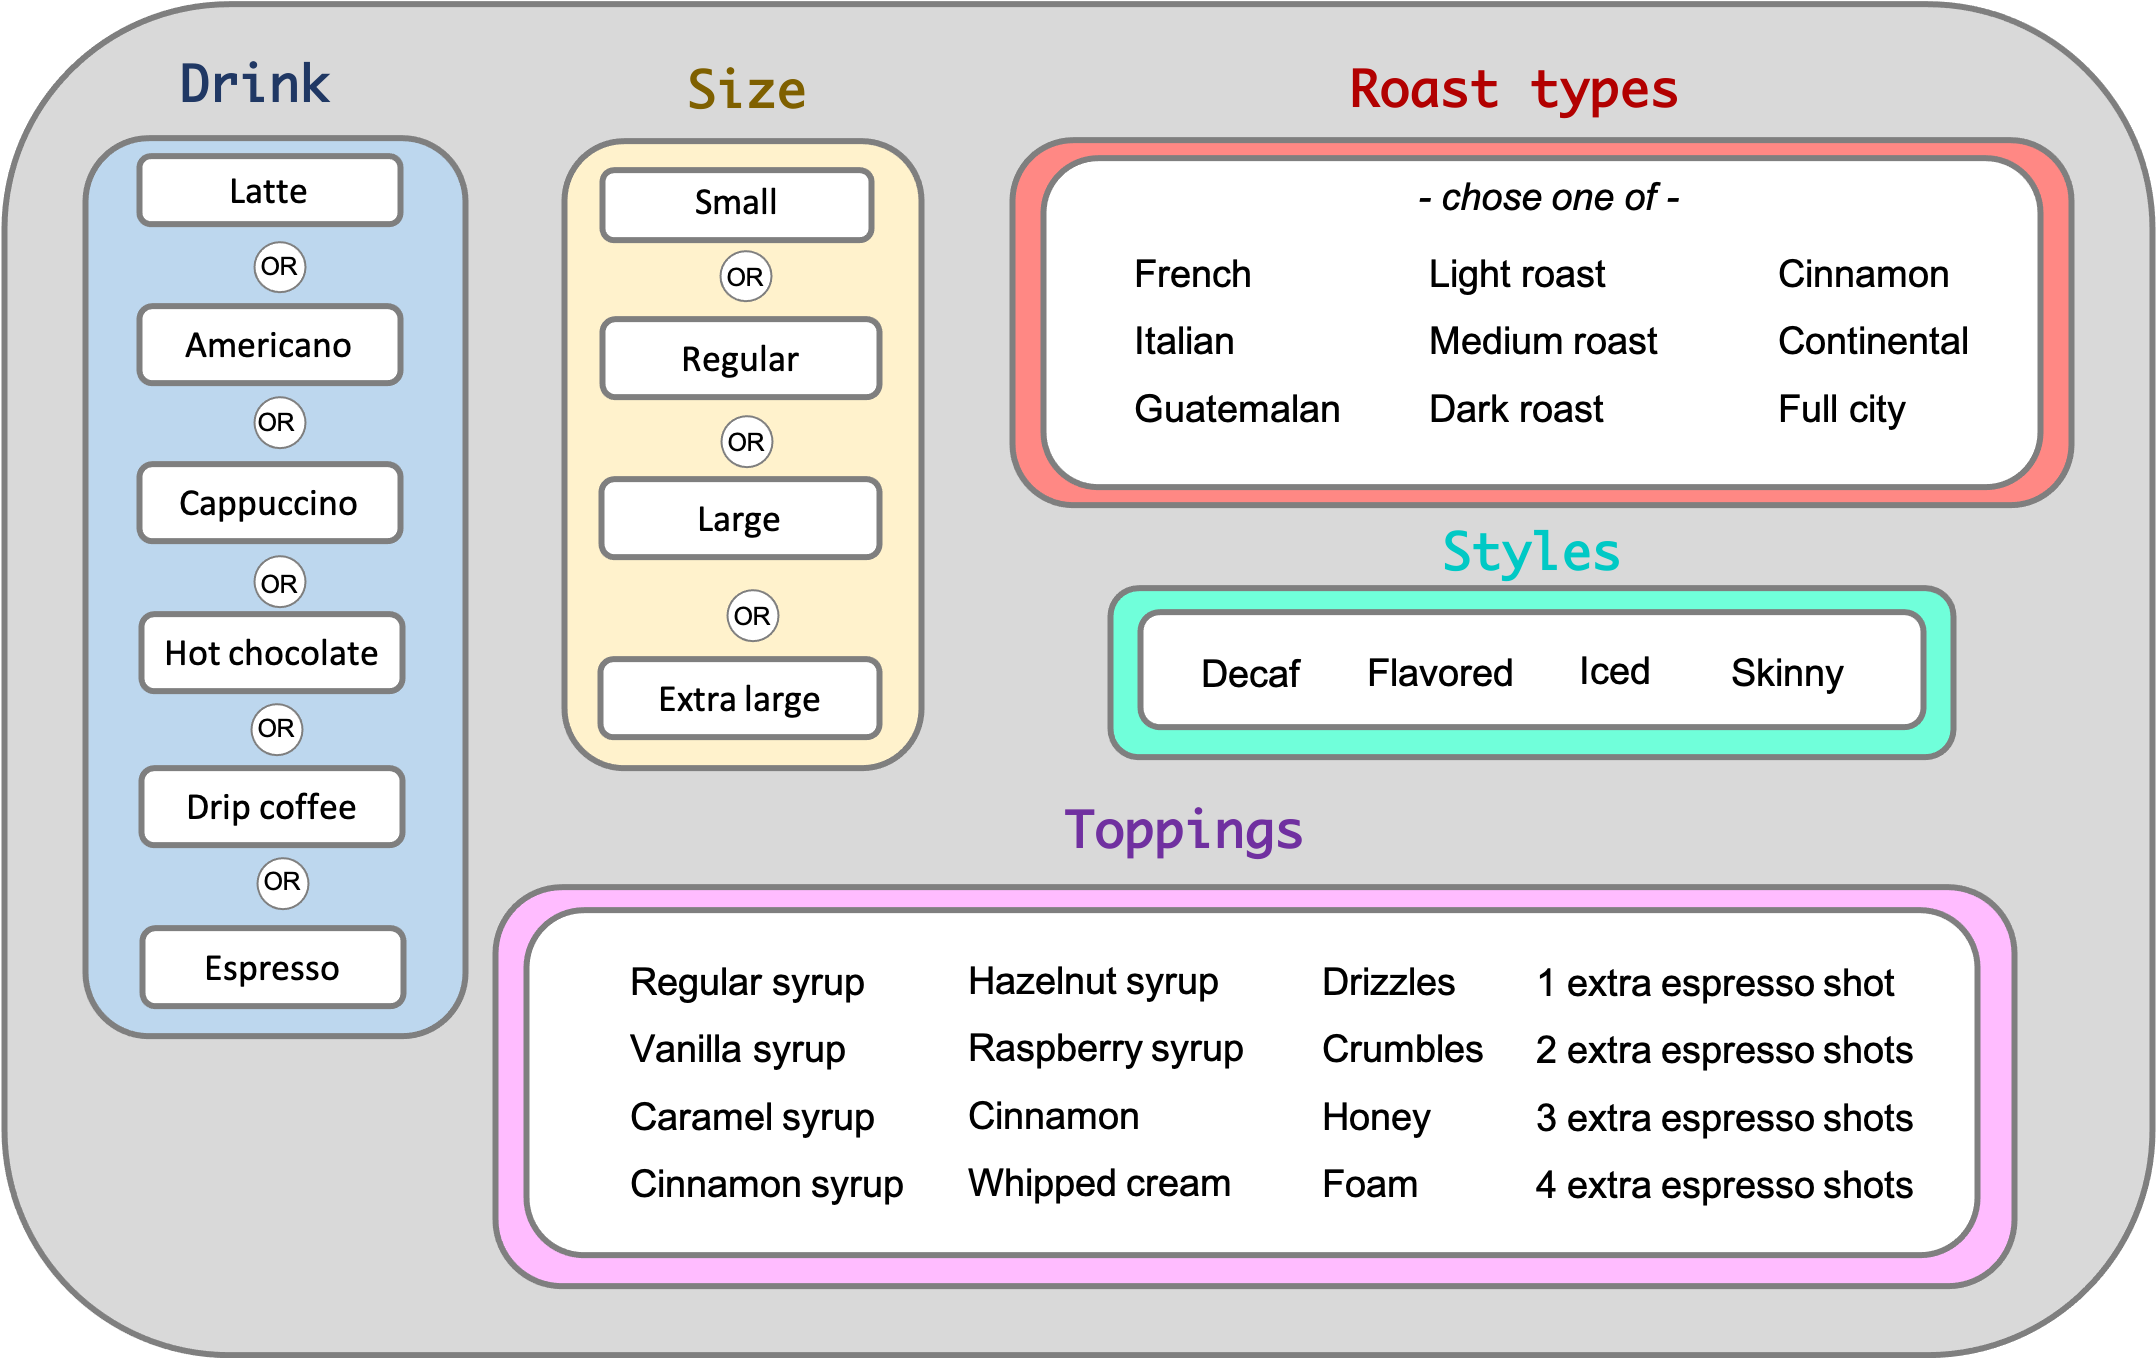}
	\end{subfigure}
	\caption{Menus shown to MTurk workers for each task: \textsc{burrito} (top-left), \textsc{Sub} (top-right), \textsc{Burger} (bottom-left) and \textsc{coffee} (bottom-right) ).}\label{fig:allMenus}
\end{figure*}

\newpage
\section{Skill schemas}\label{appendix:skillSchemas}

In figure \ref{fig:allSchema} we provide the detailed skill schema for each skill, which describe the intents anmes, slots names, slots properties, and intents slots dependencies. The actual catalog values for each slot will be released as part of our dataset release.

\medskip

\begin{figure*}[b]
\tiny
	\centering
	\begin{minipage}{0.5\textwidth}
	\begin{subfigure}[b]{0.8\textwidth}	
	\begin{lstlisting}[language=json]
{
  "name":  "PIZZA"
  "intents":  [
    {"name": "PIZZAORDER",
      "slots": [
        {"name": "NUMBER"},
        {"name": "SIZE"},
        {"name": "STYLE"},
        {"name": "TOPPING",
          "negatable": true,
          "quantifiable":  true}
        ]
    },
    {"name": "DRINKORDER",
      "slots": [
        {"name": "NUMBER"},
        {"name": "SIZE"},
        {"name": "VOLUME"},
        {"name": "DRINKTYPE"},
        {"name": "CONTAINERTYPE"}
]}]}
	\end{lstlisting}
	\end{subfigure}
\vskip\baselineskip
	\begin{subfigure}[b]{0.8\textwidth}
		\begin{lstlisting}[language=json]
{
"name": "SUB",
"intents":  [
 {"name": "SANDWICH_ORDER",
   "slots": [
     {"name": "NUMBER"},
     {"name": "BASE_SANDWICH"},
     {"name": "TOPPING",
       "negatable": true,
       "quantifiable":  true}
   ]
 },
 {"name": "SIDE_ORDER",
   "slots": [
     {"name": "NUMBER"},
     {"name": "SIDE_TYPE"}
   ]
 },
 {"name": "DRINK_ORDER",
   "slots": [
     {"name": "NUMBER"},
     {"name": "DRINK_TYPE"}
]}]}
		\end{lstlisting}
			\end{subfigure}
\vskip\baselineskip
	\begin{subfigure}[b]{0.8\textwidth}
	\begin{lstlisting}[language=json]
{
  "name": "BURGER",
  "intents":  [
    {"name": "MAIN_DISH_ORDER",
      "slots": [
        {"name": "NUMBER"},
        {"name": "MAIN_DISH_TYPE"},
        {"name": "TOPPING",
          "negatable": true,
          "quantifiable":  true}
      ]
    },
    {"name": "SIDE_ORDER",
      "slots": [
        {"name": "NUMBER"},
        {"name": "SIDE_TYPE"},
        {"name": "SIZE"}
      ]
    },
    {"name": "DRINK_ORDER",
      "slots": [
        {"name": "NUMBER"},
        {"name": "DRINK_TYPE"},
        {"name": "SIZE"}
]}]}
	\end{lstlisting}
\end{subfigure}
\vskip\baselineskip
	\begin{subfigure}[b]{0.8\textwidth}
	\begin{lstlisting}[language=json]
{
  "name": "COFFEE",
  "intents":  [
    {"name": "DRINK_ORDER",
      "slots": [
        {"name": "NUMBER"},
        {"name": "SIZE"},
        {"name": "STYLE"},
        {"name": "NUMBER"},
        {"name": "ROAST_TYPE"},
        {"name": "DRINK_TYPE"},
        {"name": "TOPPING",
          "negatable": true,
          "quantifiable":  true}
]}]}
	\end{lstlisting}
\end{subfigure}
\end{minipage}%
\begin{minipage}{0.6\textwidth}
	\tiny
	\begin{subfigure}[b]{\textwidth}	
	\begin{lstlisting}[language=json]
{
  "name": "BURRITO",
  "intents":  [
    {"name": "BURRITO_ORDER",
      "slots": [ 
      {"name": "NUMBER"}, {"name": "MAIN_FILLING", "quantifiable":  true}, 
      {"name": "RICE_FILLING", "negatable": true, "quantifiable":  true},
      {"name": "BEAN_FILLING", "negatable": true, "quantifiable":  true}, 
      {"name": "SALSA_TOPPING", "negatable": true, "quantifiable":  true},
      {"name": "TOPPING", "negatable": true, "quantifiable":  true}
      ]
    },
    {"name": "BURRITO_BOWL_ORDER",
      "slots": [ 
      {"name": "NUMBER"}, {"name": "MAIN_FILLING", "quantifiable":  true}, 
      {"name": "RICE_FILLING", "negatable": true, "quantifiable":  true},
      {"name": "BEAN_FILLING", "negatable": true, "quantifiable":  true}, 
      {"name": "SALSA_TOPPING", "negatable": true, "quantifiable":  true},
      {"name": "TOPPING", "negatable": true, "quantifiable":  true}
      ]
    },
    {"name": "SALAD_ORDER",
      "slots": [ 
      {"name": "NUMBER"}, {"name": "MAIN_FILLING", "quantifiable":  true}, 
      {"name": "RICE_FILLING", "negatable": true, "quantifiable":  true},
      {"name": "BEAN_FILLING", "negatable": true, "quantifiable":  true}, 
      {"name": "SALSA_TOPPING", "negatable": true, "quantifiable":  true},
      {"name": "TOPPING", "negatable": true, "quantifiable":  true}
      ]
    },
    {"name": "TACO_ORDER",
      "slots": [ 
      {"name": "NUMBER"}, {"name": "MAIN_FILLING", "quantifiable":  true}, 
      {"name": "RICE_FILLING", "negatable": true, "quantifiable":  true},
      {"name": "BEAN_FILLING", "negatable": true, "quantifiable":  true}, 
      {"name": "SALSA_TOPPING", "negatable": true, "quantifiable":  true},
      {"name": "TOPPING", "negatable": true, "quantifiable":  true}
      ]
    },
    {"name": "QUESADILLA_ORDER",
      "slots": [ 
      {"name": "NUMBER"}, {"name": "MAIN_FILLING", "quantifiable":  true}, 
      {"name": "RICE_FILLING", "negatable": true, "quantifiable":  true},
      {"name": "BEAN_FILLING", "negatable": true, "quantifiable":  true}, 
      {"name": "SALSA_TOPPING", "negatable": true, "quantifiable":  true},
      {"name": "TOPPING", "negatable": true, "quantifiable":  true}
      ]
    },
    {"name": "SIDE_ORDER",
      "slots": [
        {"name": "NUMBER"},
        {"name": "SIDE_TYPE"},
        {"name": "SALSA_TOPPING", "negatable": true, "quantifiable":  true}
      ]
    },
    {"name": "DRINK_ORDER",
      "slots": [
        {"name": "NUMBER"},
        {"name": "DRINK_TYPE"}
      ]
    }
  ]
}
	\end{lstlisting}
\end{subfigure}
\caption{Skill schema for the five food skills.}\label{fig:allSchema}
\end{minipage}
\end{figure*}

\textsc{note}: it can be noticed that not all schemas have the same available slots for similar intents. For example the \textsc{burger} skill has a \textsc{size} attribute for the \texttt{DRINK\_ORDER} and \texttt{SIDE\_ORDER} intents, while the \textsc{burrito} skill does not. This is a design choice meant to reflect a real-life situation where the person desigining the schema might or might no choose to add such propertie if it cannot be supported by the back-end or is simply not available in pre-existing menu. As a consequence it will be found that in the \textsc{burrito} dataset if the request is for \emph{"a chicken burrito with one small diet coke"} then the EXR labeling will not contain \texttt{(SIZE small )} for the drink. This is a supplementary difficulty for our models, and a challenge of these realistically customer defined schemas.

\section{Data examples}\label{appendix:dataExamples}
In table \ref{table:exmap} we provide examples of the collected utterances, and their linearized semantics obtained form internal annotators. As can be seen in the table, uttterances have varying degrees of complexities, which results in linearized trees of varying depths and width.
 
\begin{table*}[!hbt]
  \centering {\scriptsize   
	\begin{tabular}{|l|l||l|}
		\hline
		\textbf{Datset} & \textbf{Natural Language} & 	\textbf{EXR Linearized Semantics} \\	\hline
		 \textsc{pizza} &\makecell[l]{five medium pizzas with tomatoes \\ and ham} & \makecell[l]{\smtt{(PIZZAORDER} \\ \smtt{(NUMBER 5 )} \smtt{(SIZE medium )} \\ \smtt{(TOPPING ham )} \smtt{(TOPPING tomatoes ))} } \\ \hline
		\textsc{pizza} &\makecell[l]{i'll have one pie along with pesto and ham  \\ but avoid olives.} & \makecell[l]{\smtt{(PIZZAORDER} \\ \smtt{(NOT (TOPPING olives ) )} \\ \smtt{(NUMBER 1 )} \smtt{(TOPPING ham )} \smtt{(TOPPING pesto ))}}  \\  \hline
		\textsc{pizza} &\makecell[l]{i wanted to have two dr peppers three \\ pepsis and a sprite.} & \makecell[l]{\smtt{(DRINKORDER} \smtt{(DRINKTYPE dr\_pepper )} \smtt{(NUMBER 2 ))} \\ \smtt{(DRINKORDER} \smtt{(DRINKTYPE pepsi )} \smtt{(NUMBER 3 ))} \\ \smtt{(DRINKORDER} \smtt{(DRINKTYPE sprite )} \smtt{(NUMBER 1 ))} } \\ \hline
		 \textsc{burrito} &\makecell[l]{burrito with steak cheese guacamole sour \\ cream and fresh tomato salsa} & \makecell[l]{\smtt{(BURRITO\_ORDER} \\ \smtt{(NUMBER 1 )} \smtt{(MAIN\_FILLING steak )} \\ \smtt{(TOPPING cheese ) (TOPPING guacamole )} \\ \smtt{(TOPPING sour\_cream )} \\ \smtt{(SALSA\_TOPPING fresh\_tomato\_salsa ) )} } \\ \hline
		\textsc{burrito} &\makecell[l]{i'd also like a bottled water please.} & \makecell[l]{\smtt{(DRINK\_ORDER} \\ \smtt{(NUMBER 1 )} \smtt{(DRINK\_TYPE bottled\_water ))}}  \\  \hline
		\textsc{burrito} & \makecell[l]{i'd like a lemonade with a side of chips.} & \makecell[l]{\smtt{(DRINK\_ORDER}  \\ \smtt{(NUMBER 1 )} \smtt{(DRINK\_TYPE tractor\_lemonade )} \\ \smtt{(SIDE\_ORDER} \\ \smtt{(NUMBER 1 )} \smtt{(SIDE\_TYPE chips ))} } \\ \hline
		\textsc{sub} & \makecell[l]{steak and cheese sandwich with lettuce \\ cucumbers and olives}  & \makecell[l]{ \smtt{(SANDWICH\_ORDER (NUMBER 1 ) } \\ \smtt{(BASE\_SANDWICH steak\_and\_cheese )} \\ \smtt{(TOPPING lettuce ) (TOPPING cucumbers )} \\ \smtt{(TOPPING black\_olives ) )}} \\ \hline
		\textsc{sub} & \makecell[l]{i will order a chicken and bacon ranch \\ sandwich  and on that please put \\ american cheese chipotle southwest sauce \\  lettuce tomatoes pickles with a side \\ of doritos and two chocolate chip cookies} &  \makecell[l]{ \smtt{(SANDWICH\_ORDER (NUMBER 1 )} \\ \smtt{(BASE\_SANDWICH chicken\_and\_bacon\_ranch ) } \\  \smtt{(TOPPING american\_cheese )} \\ \smtt{(TOPPING chipotle\_southwest )} \\  \smtt{(TOPPING lettuce ) (TOPPING tomatoes )} \\  \smtt{(TOPPING pickles ) )} \\  \smtt{(SIDE\_ORDER (NUMBER 1 )} \\  \smtt{(SIDE\_TYPE doritos\_nacho\_cheese ) )} \\  \smtt{(SIDE\_ORDER (NUMBER 2 )} \\  \smtt{(SIDE\_TYPE chocolate\_chip ) )}} \\ \hline
		\textsc{burger} & \makecell[l]{hi can i have the double cheeseburger \\ with ketchup and onions and french fries \\ on the side} &  \makecell[l]{ \smtt{(MAIN\_DISH\_ORDER (NUMBER 1 ) } \\ \smtt{(MAIN\_DISH\_TYPE double\_cheese\_burger )} \\  \smtt{(TOPPING ketchup ) (TOPPING onion ) )} \\ \smtt{(SIDE\_ORDER (NUMBER 1 )} \\  \smtt{(SIDE\_TYPE french\_fries ) )} } \\ \hline
		\textsc{burger} & \makecell[l]{veggie burger with lettuce and bacon \\  large curly fry and a small iced tea} &  \makecell[l]{ \smtt{(MAIN\_DISH\_ORDER (NUMBER 1 )} \\  \smtt{(MAIN\_DISH\_TYPE vegan\_burger )} \\  \smtt{(TOPPING lettuce ) (TOPPING bacon )  )} \\ \smtt{(SIDE\_ORDER (NUMBER 1 )} \\ \smtt{(SIZE large ) (SIDE\_TYPE curly\_fries ) )} \\ \smtt{(DRINK\_ORDER (NUMBER 1 )} \\ \smtt{(SIZE small ) (DRINK\_TYPE iced\_tea ) )}} \\ \hline
		\textsc{coffee} & \makecell[l]{i'd like a large hot chocolate with \\ whipped cream} &   \makecell[l]{ \smtt{(DRINK\_ORDER} \\  \smtt{(NUMBER 1 ) (SIZE large )} \\ \smtt{(DRINK\_TYPE hot\_chocolate )} \\  \smtt{(TOPPING whipped\_cream ) )}} \\ \hline
		\textsc{coffee} & \makecell[l]{one regular latte light roast with an \\ extra espresso shot and honey added and \\ one large cappuccino with caramel syrup \\ in that one} & \makecell[l]{ \smtt{(DRINK\_ORDER (NUMBER 1 )} \\ \smtt{(SIZE regular ) (DRINK\_TYPE latte )} \\ \smtt{(ROAST\_TYPE light\_roast ) (TOPPING honey )} \\ \smtt{(TOPPING (ESPRESSO\_SHOT 1 ) ) )} \\ \smtt{(DRINK\_ORDER (NUMBER 1 )} \\ \smtt{(SIZE large ) (DRINK\_TYPE cappuccino )} \\ \smtt{(TOPPING caramel\_syrup ) )} } \\ \hline
		
	\end{tabular}
}        
	\caption{Example nautral language utterances obtained from Mechanical Turk tasks and annotation given by internal labelers.} \label{table:exmap}
\end{table*}

\section{Syntehtic data generation templates}\label{appendix:synth}
In table \ref{table:synthEx} we examplify the templates used for data generation by showing 4 of the used templates for generating synthetic data for the \textsc{sub} and \textsc{burrito} datasets. For \textsc{sub} we used 32 templates and for \textsc{burrito} we used 46.

\begin{table*}[!hbt]
  \centering {\scriptsize   
	\begin{tabular}{|l|l||l|}
		\hline
		\textbf{Datset} & \textbf{Template} & 	\textbf{Example catalog values} \\	\hline
		\textsc{sub} & \makecell[l]{ \smtt{ \{prelude\} \{number\} \{side\_type\} } }   &  \makecell[l]{ \smtt{\{prelude\}} = \textit{i want to order} \\  \smtt{\{side\_type\} } = \textit{sunchips} }  \\ \hline
		\textsc{sub} & \makecell[l]{  \smtt{ \{prelude\} \{number\} \{base\_sandwich\} with} \\  \smtt{\{topping1\} and \{topping2\} } } &  \makecell[l]{ \smtt{\{base\_sandwich\}} = \textit{chicken teriyaki} \\  \smtt{\{topping1\} } = \textit{bacon} } \\ \hline
		\textsc{burrito} & \makecell[l]{ \smtt{ \{prelude\} \{number\} \{main\_filling\} \{entity\_name\} } \\ \smtt{ with \{salsa\_topping\} }  } &   \makecell[l]{ \smtt{\{main\_filling\}} = \textit{barbacoa} \\  \smtt{\{entity\_name\} } = \textit{burrito} } \\ \hline
		\textsc{burrito} & \makecell[l]{ \smtt{\{prelude\} \{number\} side of \{side\_type1\} and} \\ \smtt{ \{side\_type2\} and \{number\} \{drink\_type\} } } & \makecell[l]{ \smtt{\{side\_type1\}} = \textit{chips} \\  \smtt{\{side\_type2\} } = \textit{guac} } \\ \hline
	\end{tabular}
}        
	\caption{Example templates and catalog values used for sampling synthetic data.} \label{table:synthEx}
\end{table*}
